# Supplementary material for: Selection of a representative sorting model in a preference disaggregation setting: a review of existing procedures, new proposals, and experimental comparison
Source: arXiv:2209.02410 ancillary file (2022-08-30)
Supplement: Supplementary file 1 [file eAppendix.pdf]

# Selection of a representative sorting model in a preference disaggregation setting: a review of existing procedures, new proposals, and experimental comparison

Michał Wójcik[a], Miłosz Kadziński[a], Krzysztof Ciomek[a]

[a]*Institute of Computing Science, Poznan University of Technology, Piotrowo 2, 60-965 Poznań, Poland*

## 1. Experimental results concerning differences between marginal and comprehensive values and class thresholds

In this section, we consider the outcomes concerning the differences between the reference and resulting models obtained for different values of each problem dimension ($p$, $m$, $\gamma_j$, and $R$).

### 1.1. Differences between marginal values

An increase in the number of classes has a positive effect on reproducing the DM's preference model in terms of marginal values (see Table 1). This is confirmed for all procedures. The monotonicity of the decrease in differences is the greatest between 2- and 3-class problems. Furthermore, UTADISMP1 and ROBUST-ITER (both attain 0.1009 for 2-class and 0.0313 for 5-class instances) improve most significantly with the increase of $p$. However, for 2-class problems, these two methods are only better than MAX-SVF (0.2053) and MIN-SVF (0.1436), whereas, for 5-class problems, their results are only slightly worse than for REPDIS (0.0291) and the center-based approaches (0.0253 for ACUTADIS and 0.0287 for CHEBYSHEV).

Table 1: Average differences between marginal values for various numbers of classes.

| | Reference | | | | Centroid | | | |
|---|---|---|---|---|---|---|---|---|
| **Procedure** | **2** | **3** | **4** | **5** | **2** | **3** | **4** | **5** |
| UTADISMP1 | 0.1009 | 0.0591 | 0.0413 | 0.0313 | 0.0933 | 0.0495 | 0.0318 | 0.0227 |
| UTADISMP2 | 0.0971 | 0.0616 | 0.0466 | 0.0370 | 0.0867 | 0.0522 | 0.0381 | 0.0293 |
| UTADISMP3 | 0.0819 | 0.0648 | 0.0531 | 0.0430 | 0.0495 | 0.0463 | 0.0401 | 0.0337 |
| UTADIS-JLS | 0.0841 | 0.0601 | 0.0446 | 0.0345 | 0.0611 | 0.0457 | 0.0356 | 0.0279 |
| CHEBYSHEV | 0.0697 | 0.0484 | 0.0368 | 0.0287 | 0.0320 | 0.0222 | 0.0163 | 0.0123 |
| MAX-SVF | 0.2052 | 0.1496 | 0.1112 | 0.0833 | 0.2067 | 0.1508 | 0.1118 | 0.0830 |
| MIN-SVF | 0.1435 | 0.1083 | 0.0840 | 0.0654 | 0.1420 | 0.1071 | 0.0821 | 0.0642 |
| MSCVF | 0.0953 | 0.0645 | 0.0496 | 0.0417 | 0.0832 | 0.0550 | 0.0432 | 0.0374 |
| ACUTADIS | 0.0650 | 0.0440 | 0.0326 | 0.0253 | 0.0336 | 0.0255 | 0.0202 | 0.0162 |
| CENTROID | 0.0672 | 0.0469 | 0.0358 | 0.0280 | 0 | 0 | 0 | 0 |
| REPDIS | 0.0777 | 0.0519 | 0.0381 | 0.0291 | 0.0471 | 0.0268 | 0.0170 | 0.0117 |
| CAI | 0.0883 | 0.0697 | 0.0553 | 0.0434 | 0.0633 | 0.0510 | 0.0399 | 0.0309 |
| APOI | 0.0886 | 0.0698 | 0.0556 | 0.0436 | 0.0634 | 0.0511 | 0.0401 | 0.0312 |
| COMB | 0.0886 | 0.0698 | 0.0556 | 0.0436 | 0.0634 | 0.0511 | 0.0401 | 0.0312 |
| ROBUST-ITER | 0.1009 | 0.0591 | 0.0413 | 0.0313 | 0.0933 | 0.0495 | 0.0318 | 0.0227 |
| ROBUST-COMP | 0.0981 | 0.0628 | 0.0470 | 0.0374 | 0.0884 | 0.0546 | 0.0408 | 0.0326 |

A higher number of criteria also reduces a gap between marginal values (see Table 2). This is understandable because, with more criteria, their shares in the comprehensive values decrease, leading to the lesser differences between the compared models. The most substantial differences for the extreme numbers of criteria can be observed for UTADISMP3 and UTADIS-JLS. For both approaches, the mean differences between marginal values decreased more than two times when comparing problems with three and nine criteria (for UTADISMP3 - from 0.0873 to 0.0421, and for UTADIS-JLS – from 0.0822 to 0.0390). With a greater number of criteria, their solutions become more similar to the central models, which approximate the DM's preferences up to a satisfactory level.

*Email addresses:* `michal.wojcik@cs.put.poznan.pl` (Michał Wójcik), `milosz.kadzinski@cs.put.poznan.pl` (Miłosz Kadziński), `k.ciomek@gmail.com` (Krzysztof Ciomek)

Table 2: Average differences between marginal values for various numbers of criteria.

| | Reference | | | | Centroid | | | |
|---|---|---|---|---|---|---|---|---|
| **Procedure** | **3** | **5** | **7** | **9** | **3** | **5** | **7** | **9** |
| UTADISMP1 | 0.0748 | 0.0596 | 0.0516 | 0.0467 | 0.0594 | 0.0509 | 0.0454 | 0.0416 |
| UTADISMP2 | 0.0825 | 0.0619 | 0.0519 | 0.0461 | 0.0681 | 0.0524 | 0.0452 | 0.0406 |
| UTADISMP3 | 0.0873 | 0.0632 | 0.0502 | 0.0421 | 0.0636 | 0.0438 | 0.0342 | 0.0279 |
| UTADIS-JLS | 0.0822 | 0.0566 | 0.0455 | 0.0390 | 0.0644 | 0.0423 | 0.0340 | 0.0295 |
| CHEBYSHEV | 0.0621 | 0.0474 | 0.0395 | 0.0346 | 0.0296 | 0.0215 | 0.0172 | 0.0146 |
| MAX-SVF | 0.1896 | 0.1425 | 0.1172 | 0.0999 | 0.1939 | 0.1428 | 0.1165 | 0.0991 |
| MIN-SVF | 0.1406 | 0.1041 | 0.0846 | 0.0720 | 0.1399 | 0.1022 | 0.0830 | 0.0704 |
| MSCVF | 0.0837 | 0.0645 | 0.0548 | 0.0481 | 0.0670 | 0.0567 | 0.0503 | 0.0448 |
| ACUTADIS | 0.0560 | 0.0430 | 0.0362 | 0.0316 | 0.0328 | 0.0247 | 0.0204 | 0.0176 |
| CENTROID | 0.0591 | 0.0459 | 0.0388 | 0.0342 | 0 | 0 | 0 | 0 |
| REPDIS | 0.0681 | 0.0497 | 0.0420 | 0.0371 | 0.0381 | 0.0246 | 0.0208 | 0.0191 |
| CAI | 0.0897 | 0.0669 | 0.0542 | 0.0459 | 0.0663 | 0.0478 | 0.0385 | 0.0325 |
| APOI | 0.0901 | 0.0670 | 0.0544 | 0.0460 | 0.0668 | 0.0479 | 0.0387 | 0.0325 |
| COMB | 0.0901 | 0.0670 | 0.0544 | 0.0460 | 0.0668 | 0.0479 | 0.0387 | 0.0325 |
| ROBUST-ITER | 0.0748 | 0.0596 | 0.0516 | 0.0467 | 0.0593 | 0.0509 | 0.0454 | 0.0416 |
| ROBUST-COMP | 0.0824 | 0.0627 | 0.0532 | 0.0471 | 0.0711 | 0.0555 | 0.0471 | 0.0427 |

The increasing number of characteristic points affects the performance of procedures differently (see Table 3). For most methods (including ROBUST-ITER, UTADISMP1, ROBUST-COMP, UTADIS-JLS, REPDIS, CAI, APOI, COMB, MAX-SVF, and MIN-SVF), an increase of $\gamma_j$ leads to a more significant difference between marginal values – and thus a deterioration in the quality of reconstructing the reference AVF (e.g., for UTADIS-JLS – the distance increases from 0.0420 to 0.0686). The center-oriented approaches (CENTROID, ACUTADIS, and CHEBYSHEV) maintain the stability of distances of their models from the reference one for different numbers of characteristic points.

The decrease of the average differences between marginal values can be observed for UTADISMP2 (0.0625 to 0.0600) and UTADISMP3 (0.0645 to 0.0569). Both approaches maximize the differences between marginal values assigned to the consecutive points. The greater the share of such values among variables optimized by the methods, the better the results achieved by these procedures. A similar trend is observed for MSCVF, which is also focused on optimizing the shape of MVFs. However, since the latter approach is applicable for settings with more than two characteristic points, in this case, the observation is confirmed only for the results obtained for instances with four and six breakpoints.

Table 3: Average differences between marginal values for various numbers of characteristic points.

| | Reference | | | Centroid | | |
|---|---|---|---|---|---|---|
| **Procedure** | **2** | **4** | **6** | **2** | **4** | **6** |
| UTADISMP1 | 0.0526 | 0.0606 | 0.0613 | 0.0391 | 0.0514 | 0.0576 |
| UTADISMP2 | 0.0625 | 0.0593 | 0.0600 | 0.0537 | 0.0466 | 0.0544 |
| UTADISMP3 | 0.0645 | 0.0607 | 0.0569 | 0.0571 | 0.0398 | 0.0303 |
| UTADIS-JLS | 0.0420 | 0.0570 | 0.0686 | 0.0249 | 0.0453 | 0.0576 |
| CHEBYSHEV | 0.0446 | 0.0469 | 0.0462 | 0.0272 | 0.0206 | 0.0144 |
| MAX-SVF | 0.0921 | 0.1386 | 0.1813 | 0.0892 | 0.1403 | 0.1848 |
| MIN-SVF | 0.0929 | 0.0999 | 0.1081 | 0.0891 | 0.0993 | 0.1082 |
| MSCVF | | 0.0664 | 0.0591 | | 0.0574 | 0.0521 |
| ACUTADIS | 0.0416 | 0.0424 | 0.0410 | 0.0225 | 0.0262 | 0.0229 |
| CENTROID | 0.0393 | 0.0474 | 0.0467 | 0 | 0 | 0 |
| REPDIS | 0.0426 | 0.0522 | 0.0528 | 0.0214 | 0.0262 | 0.0293 |
| CAI | 0.0508 | 0.0690 | 0.0727 | 0.0362 | 0.0494 | 0.0532 |
| APOI | 0.0510 | 0.0693 | 0.0729 | 0.0367 | 0.0495 | 0.0532 |
| COMB | 0.0510 | 0.0693 | 0.0729 | 0.0367 | 0.0495 | 0.0532 |
| ROBUST-ITER | 0.0526 | 0.0606 | 0.0613 | 0.0391 | 0.0514 | 0.0575 |
| ROBUST-COMP | 0.0526 | 0.0638 | 0.0677 | 0.0414 | 0.0566 | 0.0643 |

The impact of different numbers of reference alternatives per class is reported in Table 4. With richer preference information, the differences between marginal values become lesser for all procedures. Again, the change in the number of reference alternatives has the greatest impact on the performance of UTADISMP1 and ROBUST-ITER (compare 8.26% for $R = 3$ and 4.01% for $R = 10$). Interestingly, for CAI, APOI, and COMB, the relative distances from the centroid solution are stable for different values of $R$. However, their distances from the reference model decrease when additional assignment examples become available.

Table 4: Average differences between marginal values for various numbers of reference alternatives per class.

| | Reference | | | | Centroid | | | |
|---|---|---|---|---|---|---|---|---|
| **Procedure** | **3** | **5** | **7** | **10** | **3** | **5** | **7** | **10** |
| UTADISMP1 | 0.0826 | 0.0609 | 0.0491 | 0.0401 | 0.0749 | 0.0516 | 0.0399 | 0.0309 |
| UTADISMP2 | 0.0824 | 0.0629 | 0.0527 | 0.0443 | 0.0738 | 0.0536 | 0.0434 | 0.0355 |
| UTADISMP3 | 0.0749 | 0.0641 | 0.0558 | 0.0480 | 0.0503 | 0.0446 | 0.0398 | 0.0349 |
| UTADIS-JLS | 0.0745 | 0.0590 | 0.0493 | 0.0405 | 0.0573 | 0.0450 | 0.0373 | 0.0307 |
| CHEBYSHEV | 0.0594 | 0.0484 | 0.0410 | 0.0349 | 0.0272 | 0.0217 | 0.0184 | 0.0156 |
| MAX-SVF | 0.1846 | 0.1461 | 0.1209 | 0.0977 | 0.1853 | 0.1470 | 0.1215 | 0.0986 |
| MIN-SVF | 0.1299 | 0.1064 | 0.0901 | 0.0748 | 0.1283 | 0.1050 | 0.0885 | 0.0735 |
| MSCVF | 0.0843 | 0.0646 | 0.0549 | 0.0473 | 0.0746 | 0.0559 | 0.0473 | 0.0410 |
| ACUTADIS | 0.0535 | 0.0440 | 0.0373 | 0.0320 | 0.0268 | 0.0246 | 0.0228 | 0.0213 |
| CENTROID | 0.0577 | 0.0467 | 0.0397 | 0.0339 | 0 | 0 | 0 | 0 |
| REPDIS | 0.0621 | 0.0513 | 0.0449 | 0.0385 | 0.0286 | 0.0265 | 0.0249 | 0.0225 |
| CAI | 0.0742 | 0.0668 | 0.0604 | 0.0553 | 0.0492 | 0.0481 | 0.0452 | 0.0426 |
| APOI | 0.0747 | 0.0670 | 0.0606 | 0.0553 | 0.0497 | 0.0482 | 0.0454 | 0.0426 |
| COMB | 0.0746 | 0.0670 | 0.0606 | 0.0553 | 0.0497 | 0.0481 | 0.0454 | 0.0426 |
| ROBUST-ITER | 0.0826 | 0.0609 | 0.0491 | 0.0401 | 0.0749 | 0.0516 | 0.0399 | 0.0309 |
| ROBUST-COMP | 0.0821 | 0.0644 | 0.0535 | 0.0454 | 0.0757 | 0.0565 | 0.0459 | 0.0384 |

### *1.2. Differences between comprehensive values*

A greater number of classes has a positive effect on reproducing the original comprehensive values assigned by the DM to alternatives (see Table 5). The ACUTADIS method turns out to be the best irrespective of $p$ (0.0727 for 2-class and 0.0337 for 5-class problem instances). On the contrary, the most considerable relative differences can be observed for UTADISMP1 and ROBUST-ITER (the difference between comprehensive decreases from 0.1434 to 0.0434 when moving from 2 to 5 classes). The methods optimizing the sum of comprehensive values attain the worst results. This means that putting all alternatives in the best or the worst possible light, as done by MAX-SVF and MIX-SVF, does not correspond with the assessments conducted in the DM's reference models, where the characteristics of these comprehensive evaluations are more diverse.

Table 5: Average differences between comprehensive values for various numbers of classes.

| **Procedure** | **2** | **3** | **4** | **5** |
|---|---|---|---|---|
| UTADISMP1 | 0.1434 | 0.0807 | 0.0568 | 0.0434 |
| UTADISMP2 | 0.1380 | 0.0791 | 0.0579 | 0.0460 |
| UTADISMP3 | 0.0835 | 0.0695 | 0.0587 | 0.0501 |
| UTADIS-JLS | 0.1531 | 0.1054 | 0.0790 | 0.0611 |
| CHEBYSHEV | 0.0773 | 0.0589 | 0.0470 | 0.0381 |
| MAX-SVF | 0.3037 | 0.2578 | 0.2154 | 0.1794 |
| MIN-SVF | 0.3026 | 0.2581 | 0.2161 | 0.1794 |
| MSCVF | 0.1178 | 0.0887 | 0.0748 | 0.0665 |
| ACUTADIS | 0.0727 | 0.0532 | 0.0412 | 0.0337 |
| CENTROID | 0.0760 | 0.0580 | 0.0463 | 0.0378 |
| REPDIS | 0.0935 | 0.0661 | 0.0497 | 0.0394 |
| CAI | 0.1553 | 0.0938 | 0.0664 | 0.0511 |
| APOI | 0.1541 | 0.0933 | 0.0649 | 0.0508 |
| COMB | 0.1541 | 0.0933 | 0.0650 | 0.0508 |
| ROBUST-ITER | 0.1434 | 0.0806 | 0.0568 | 0.0434 |
| ROBUST-COMP | 0.1383 | 0.0853 | 0.0646 | 0.0529 |

An increase in the number of criteria differently influences the results of particular methods (see Table 6). A greater number of performance dimensions positively affects the performance of UTADISMP3, MSCVF, CHEBYSHEV, ACUTADIS, CENTROID and REPDIS. The greatest relative differences between 3- and 9-attribute problems are observed for UTADISMP3 (from 7.22% to 5.98%) and REPDIS (from 7.05% to 5.85%). In general, these methods optimize the shape of MCVFs or exploit the geometry of the polyhedron of all feasible models. On the contrary, with a more significant number of criteria, the average difference from the reference model in terms of comprehensive values increases for UTADISMP1, UTADISMP2, MAX-SVF, MIN-SVF, CAI, APOI, COMB, and ROBUST-ITER. These approaches focus on optimizing the comprehensive values of alternatives, usually making them as discriminatory as possible, though based on differently formulated objectives.

Table 7 shows that for the vast majority of procedures, adding characteristic points leads to an increased difference between comprehensive values. The most significant increase is observed between instances with two and four characteristic points (e.g., for MAX-SVF – the respective values are 0.0626 and 0.2843). The central-based approaches also record relatively

Table 6: Average differences between comprehensive values for various numbers of criteria.

| Procedure | 3 | 5 | 7 | 9 |
|---|---|---|---|---|
| UTADISMP1 | 0.0790 | 0.0801 | 0.0813 | 0.0838 |
| UTADISMP2 | 0.0790 | 0.0793 | 0.0802 | 0.0825 |
| UTADISMP3 | 0.0722 | 0.0672 | 0.0626 | 0.0598 |
| UTADIS-JLS | 0.1017 | 0.0941 | 0.0985 | 0.1043 |
| CHEBYSHEV | 0.0588 | 0.0561 | 0.0534 | 0.0530 |
| MAX-SVF | 0.2193 | 0.2346 | 0.2468 | 0.2556 |
| MIN-SVF | 0.2170 | 0.2351 | 0.2472 | 0.2569 |
| MSCVF | 0.0923 | 0.0876 | 0.0850 | 0.0829 |
| ACUTADIS | 0.0541 | 0.0507 | 0.0486 | 0.0475 |
| CENTROID | 0.0569 | 0.0553 | 0.0532 | 0.0528 |
| REPDIS | 0.0705 | 0.0611 | 0.0586 | 0.0585 |
| CAI | 0.0892 | 0.0907 | 0.0914 | 0.0952 |
| APOI | 0.0890 | 0.0899 | 0.0905 | 0.0937 |
| COMB | 0.0889 | 0.0899 | 0.0905 | 0.0937 |
| ROBUST-ITER | 0.0790 | 0.0801 | 0.0812 | 0.0839 |
| ROBUST-COMP | 0.0896 | 0.0851 | 0.0826 | 0.0839 |

large increases for the above instances, but this increase is already minimal when moving from four to six breakpoints. Though slightly greater in terms of absolute values, the same effect can be observed for the methods aiming at selecting the most discriminant model. In general, these results confirm that the move from linear MVFs to functions with three linear pieces increases the flexibility of the models more substantially than the change from three to five linear pieces.

Table 7: Average differences between comprehensive values for various numbers of characteristic points.

| Procedure | 2 | 4 | 6 |
|---|---|---|---|
| UTADISMP1 | 0.0359 | 0.0960 | 0.1113 |
| UTADISMP2 | 0.0404 | 0.0917 | 0.1087 |
| UTADISMP3 | 0.0413 | 0.0781 | 0.0770 |
| UTADIS-JLS | 0.0280 | 0.1109 | 0.1601 |
| CHEBYSHEV | 0.0300 | 0.0676 | 0.0684 |
| MAX-SVF | 0.0626 | 0.2843 | 0.3704 |
| MIN-SVF | 0.0632 | 0.2849 | 0.3691 |
| MSCVF | | 0.0900 | 0.0840 |
| ACUTADIS | 0.0279 | 0.0611 | 0.0617 |
| CENTROID | 0.0262 | 0.0678 | 0.0696 |
| REPDIS | 0.0280 | 0.0761 | 0.0824 |
| CAI | 0.0329 | 0.1003 | 0.1417 |
| APOI | 0.0331 | 0.1003 | 0.1389 |
| COMB | 0.0331 | 0.1003 | 0.1389 |
| ROBUST-ITER | 0.0359 | 0.0960 | 0.1113 |
| ROBUST-COMP | 0.0355 | 0.1009 | 0.1195 |

A greater number of reference alternatives per class lets all procedures construct the models that are more similar to the reference one in terms of comprehensive values (see Table 8). The largest relative decreases in differences – from 0.1165 to 0.0556 – are achieved by UTADISMP1 and ROBUST-ITER. On the contrary, the minor reduction in terms of similarities between comprehensive values is observed for CAI, APOI, and COMB (from 0.1115 to 0.0750 for CAI and from 0.1102 to 0.0745 for APOI and COMB).

### *1.3. Differences between class thresholds*

For all considered procedures, the average difference between class thresholds decreases as the number of classes increases (see Table 9). However, the level of this reduction ranges between methods. The greatest discrepancies from around 0.18 to around 0.05 are observed for methods based on robustness analysis (ROBUST-ITER and ROBUST-COMP). This is related to the fact that we consider more assignment examples with a greater number of classes. These, in turn, imply additional constraints, leading to enriched necessary inference that leaves lesser flexibility to the class thresholds when optimized by the methods. Though slightly less substantial in absolute terms, a similar trend can be observed for the CAI-based approaches. The least improvement with the increase of $p$ can be observed for UTADISMP3 and MSCVF. These approaches do not optimize the threshold values, adhering instead to a default procedure that sets the thresholds in equal distances from the extremely evaluated reference alternatives for each class.

Analogously, the average difference between class thresholds decreases when more criteria are considered (see Table 10). The exceptions hold for MAX-SVF (0.2517 for $m = 3$ and 0.2818 for $m = 9$) and the MIN-SVF (0.2518 for $m = 3$ and

Table 8: Average differences between comprehensive values for various numbers of reference alternatives per class.

| Procedure | 3 | 5 | 7 | 10 |
|---|---|---|---|---|
| UTADISMP1 | 0.1165 | 0.0839 | 0.0682 | 0.0556 |
| UTADISMP2 | 0.1130 | 0.0826 | 0.0689 | 0.0566 |
| UTADISMP3 | 0.0788 | 0.0680 | 0.0615 | 0.0536 |
| UTADIS-JLS | 0.1365 | 0.1056 | 0.0862 | 0.0704 |
| CHEBYSHEV | 0.0689 | 0.0573 | 0.0508 | 0.0443 |
| MAX-SVF | 0.2862 | 0.2491 | 0.2259 | 0.1952 |
| MIN-SVF | 0.2848 | 0.2514 | 0.2241 | 0.1959 |
| MSCVF | 0.1091 | 0.0888 | 0.0794 | 0.0706 |
| ACUTADIS | 0.0615 | 0.0521 | 0.0464 | 0.0409 |
| CENTROID | 0.0680 | 0.0566 | 0.0500 | 0.0436 |
| REPDIS | 0.0754 | 0.0642 | 0.0584 | 0.0507 |
| CAI | 0.1115 | 0.0962 | 0.0839 | 0.0750 |
| APOI | 0.1102 | 0.0950 | 0.0833 | 0.0745 |
| COMB | 0.1102 | 0.0950 | 0.0833 | 0.0745 |
| ROBUST-ITER | 0.1165 | 0.0839 | 0.0682 | 0.0556 |
| ROBUST-COMP | 0.1156 | 0.0883 | 0.0739 | 0.0632 |

Table 9: Average differences between class thresholds for various numbers of classes.

| Procedure | 2 | 3 | 4 | 5 |
|---|---|---|---|---|
| UTADISMP1 | 0.0884 | 0.0634 | 0.0475 | 0.0385 |
| UTADISMP2 | 0.0836 | 0.0622 | 0.0486 | 0.0409 |
| UTADISMP3 | 0.0595 | 0.0569 | 0.0497 | 0.0443 |
| UTADIS-JLS | 0.1459 | 0.1079 | 0.0827 | 0.0650 |
| CHEBYSHEV | 0.0583 | 0.0497 | 0.0411 | 0.0352 |
| MAX-SVF | 0.3437 | 0.2912 | 0.2383 | 0.1952 |
| MIN-SVF | 0.3421 | 0.2926 | 0.2409 | 0.1970 |
| MSCVF | 0.0928 | 0.0783 | 0.0693 | 0.0628 |
| ACUTADIS | 0.0547 | 0.0440 | 0.0346 | 0.0304 |
| CENTROID | 0.0592 | 0.0496 | 0.0407 | 0.0349 |
| REPDIS | 0.1066 | 0.0707 | 0.0533 | 0.0431 |
| CAI | 0.1390 | 0.0837 | 0.0586 | 0.0458 |
| APOI | 0.1389 | 0.0835 | 0.0570 | 0.0454 |
| COMB | 0.1388 | 0.0835 | 0.0571 | 0.0455 |
| ROBUST-ITER | 0.1828 | 0.0904 | 0.0624 | 0.0477 |
| ROBUST-COMP | 0.1720 | 0.0944 | 0.0685 | 0.0563 |

0.2838 for $m = 9$). These methods set all thresholds close to zero or one, which justifies such substantial dissimilarities. The procedures exploiting outcomes of robustness analysis do not reveal a clear monotonic trend when changing $m$. Some of them maintain a stable average difference between class thresholds in the reference and resulting models.

The results reported in Table 11 reveal a significant impact of the number of characteristic points on deviation in threshold values in relation to the reference model. Again, the most significant differences can be observed between instances with two and four breakpoints. However, when collating the outcomes for four and six characteristic points, for some approaches such as UTADISMP3, Chebyshev, MSCVF, ACUTADIS, and CENTROID, the differences are negligible, or even the trend becomes inverse. Surprisingly, for linear MVFs, MAX-SVF (0.0447) and MIN-SVF (0.0479), which have so far performed the worst in all aspects, outweigh approaches based on robustness analysis (0.0507 for ROBUST-ITER and 0.0462 for ROBUST-COMP). This is related to the fact that the latter methods try to satisfy numerous additional constraints derived from the analysis of the necessary assignment-based preference relation. Satisfying these constraints is more challenging when the only variable values that can be adjusted are the maximal share of MVFs, and it is impossible to infer convex or concave functions.

The impact of the number of reference alternatives per class on the difference between class thresholds in the reference and resulting models is reported in Table 12. Clearly, these differences decrease for all methods with additional assignment examples. On the one hand, the most considerable reduction between instances with three and ten reference alternatives per class is observed for the ROBUST methods. This corresponds with the trend already explained for different numbers of classes. On the other hand, the least reductions between the extreme $R$ values are noted for the stochastic and central-based procedures. The former approaches perform rather poorly when few reference alternatives are available, and the space of compatible sorting models is large. In turn, the latter ones achieve stable, good performance regardless of the number of reference alternatives, and the enriched preference information helping them reproduce the reference model even more faithfully.

Table 10: Average differences between class thresholds for various numbers of criteria.

| **Procedure** | **3** | **5** | **7** | **9** |
|---|---|---|---|---|
| UTADISMP1 | 0.0681 | 0.0597 | 0.0553 | 0.0547 |
| UTADISMP2 | 0.0671 | 0.0592 | 0.0548 | 0.0542 |
| UTADISMP3 | 0.0661 | 0.0546 | 0.0467 | 0.0431 |
| UTADIS-JLS | 0.1143 | 0.0938 | 0.0944 | 0.0990 |
| CHEBYSHEV | 0.0581 | 0.0477 | 0.0402 | 0.0383 |
| MAX-SVF | 0.2517 | 0.2615 | 0.2735 | 0.2818 |
| MIN-SVF | 0.2518 | 0.2631 | 0.2740 | 0.2838 |
| MSCVF | 0.0914 | 0.0780 | 0.0698 | 0.0640 |
| ACUTADIS | 0.0513 | 0.0422 | 0.0363 | 0.0340 |
| CENTROID | 0.0573 | 0.0478 | 0.0406 | 0.0388 |
| REPDIS | 0.0850 | 0.0674 | 0.0617 | 0.0596 |
| CAI | 0.0831 | 0.0814 | 0.0792 | 0.0835 |
| APOI | 0.0833 | 0.0808 | 0.0787 | 0.0822 |
| COMB | 0.0833 | 0.0808 | 0.0786 | 0.0822 |
| ROBUST-ITER | 0.0990 | 0.0947 | 0.0942 | 0.0954 |
| ROBUST-COMP | 0.1113 | 0.0971 | 0.0927 | 0.0901 |

Table 11: Average differences between class thresholds for various numbers of characteristic points.

| **Procedure** | **2** | **4** | **6** |
|---|---|---|---|
| UTADISMP1 | 0.0238 | 0.0761 | 0.0785 |
| UTADISMP2 | 0.0264 | 0.0733 | 0.0767 |
| UTADISMP3 | 0.0282 | 0.0676 | 0.0620 |
| UTADIS-JLS | 0.0234 | 0.1157 | 0.1620 |
| CHEBYSHEV | 0.0214 | 0.0602 | 0.0566 |
| MAX-SVF | 0.0447 | 0.3372 | 0.4194 |
| MIN-SVF | 0.0479 | 0.3384 | 0.4182 |
| MSCVF | | 0.0803 | 0.0712 |
| ACUTADIS | 0.0180 | 0.0540 | 0.0508 |
| CENTROID | 0.0181 | 0.0615 | 0.0587 |
| REPDIS | 0.0386 | 0.0807 | 0.0860 |
| CAI | 0.0221 | 0.0914 | 0.1319 |
| APOI | 0.0227 | 0.0917 | 0.1292 |
| COMB | 0.0227 | 0.0918 | 0.1292 |
| ROBUST-ITER | 0.0507 | 0.1092 | 0.1275 |
| ROBUST-COMP | 0.0462 | 0.1120 | 0.1352 |

Table 12: Average differences between class thresholds for various numbers of reference alternatives per class.

| **Procedure** | **3** | **5** | **7** | **10** |
|---|---|---|---|---|
| UTADISMP1 | 0.0771 | 0.0623 | 0.0536 | 0.0447 |
| UTADISMP2 | 0.0755 | 0.0614 | 0.0535 | 0.0449 |
| UTADISMP3 | 0.0657 | 0.0537 | 0.0485 | 0.0425 |
| UTADIS-JLS | 0.1380 | 0.1063 | 0.0868 | 0.0704 |
| CHEBYSHEV | 0.0565 | 0.0472 | 0.0430 | 0.0376 |
| MAX-SVF | 0.3210 | 0.2790 | 0.2516 | 0.2168 |
| MIN-SVF | 0.3221 | 0.2821 | 0.2507 | 0.2178 |
| MSCVF | 0.0934 | 0.0764 | 0.0702 | 0.0632 |
| ACUTADIS | 0.0498 | 0.0421 | 0.0380 | 0.0337 |
| CENTROID | 0.0568 | 0.0475 | 0.0424 | 0.0377 |
| REPDIS | 0.0865 | 0.0714 | 0.0623 | 0.0536 |
| CAI | 0.1016 | 0.0862 | 0.0736 | 0.0658 |
| APOI | 0.1009 | 0.0853 | 0.0732 | 0.0655 |
| COMB | 0.1009 | 0.0853 | 0.0732 | 0.0655 |
| ROBUST-ITER | 0.1396 | 0.1009 | 0.0791 | 0.0636 |
| ROBUST-COMP | 0.1400 | 0.1013 | 0.0825 | 0.0674 |
